# Supplementary material for: StarGen: A Spatiotemporal Autoregression Framework with Video Diffusion Model for Scalable and Controllable Scene Generation
Source: arXiv:2501.05763 source file (2025-04-13)
Supplement: Supplementary file 1 [file X_suppl.tex]

\clearpage
\setcounter{page}{1}
\maketitlesupplementary

\section{Network Architecture}

We provide the pseudo code in~\cref{alg:code} to give a detailed explanation of the network architecture for the proposed Spatiotemporal-Conditioned Video Generation (SCVG).

\begin{algorithm}[t]

\caption{Pseudo code of the proposed SCVG.}\label{alg:code}

\lstset{style=mocov3}
\vspace{-3pt}
\begin{lstlisting}[
    language=python,
    escapechar=@,
    label=code:gslrm]
    # Input list: 
    #   spatial_images: [b, 2, h, w, 3]; b is the batch size; the spatial_images are two spatial conditioning images; h and w are the height and width
    #   temporal_images: [b, 1, h, w, 3]; the temporal conditioning image is the last temporal image of the previous prediction output;
    #   text_prompt
    #   spatial_extrinsics: [b, 2, 4, 4]; the extrinsic parameters of the three input images.
    #   spatial_intrinsics: [b, 2, 4]; the intrinsic parameters of the three input images.
    #   out_extrinsics: [b, n, 4, 4]; the extrinsic parameters. n is the frame count.
    #   out_intrinsics: [b, n, 4]; the intrinsic parameters.
    #
    # Output list:
    #   video: [b, n, h, w, 3]

    # LRM
    depths = DepthAnythingV2(spatial_images)   # [b, 2, h, w, 1]
    rays_os, rays_ds = get_rays(h, w, spatial_intrinsics, spatial_extrinsics) # rays_origin, rays_direction: [b, 2, h, w, 3]
    x = concat([spatial_images, depths, rays_ds, cross(rays_os, rays_ds)], dim=-1)     # [b, 2, h, w, 10]
    x = conv(x, out=d, kernel=8, stride=8)          # patchify to [b, 2, h/8, w/8, d]
    x = x.reshape(b, -1, d) # transformer input [b, 2 * h/8 * w/8, d]
    x = transformer(LN(x)) 
    x = LN(x)
    x = x.reshape(b*2, h//8, w//8, d)
    x = deconv(x, out=17, kernel=8, stride=8)    # [b, 2, h, w, 17]
    x = x.reshape(b, -1, 17)    # [b, 2 * h * w, 17]
    distance, feature = split(x, [1, 16], dim=-1)
    w = sigmoid(distance)
    point_cloud = rays_o + rays_d * (near * (1 - w) + far * w)
    
    # Render spatial condition
    feature_map = render(point_cloud, feature, out_extrinsic, out_intrinsic) # render feature maps from point cloud with features based on the camera's intrinsic and extrinsic parameters [b, n, h/8, w/8, 16]

    # Video Diffusion Model
    spatial_latents = causalConv3d(feature_map) # [b, n/4, h/8, w/8, 16]
    temporal_latents = vae_encode(temporal_images) #[b, 1, h/8, w/8, 16]
    control_latents = concat([temporal_latents, spatial_latents[:,1:]], dim=1) # [b, n/4, h/8, w/8, 16]
    latents = CogVideoX(noise, Controlnet(control_latents), text_prompt) # [b, n/4, h/8, w/8, 16]
    video = vae_decode(latents)

    return video
    
\end{lstlisting}\vspace{-5pt}
\end{algorithm}

\section{Additional Training Details}
We train our model using the AdamW~\cite{DBLP:conf/iclr/LoshchilovH19} optimizer with a learning rate of 0.0004. To accelerate the training process, we employ xFormers~\cite{xFormers2022} and mixed-precision~\cite{DBLP:journals/corr/abs-1710-03740} techniques. When projecting reconstructed latent features from the spatial conditioning images onto novel views, certain areas in the novel views may not be visible in the spatial conditioning images, resulting in regions without projections. During the loss calculation, we mask these regions to prevent them from influencing the loss. Our backbone is based on CogVideoX~\cite{DBLP:journals/corr/abs-2408-06072}, with the T5 model~\cite{DBLP:journals/jmlr/RaffelSRLNMZLL20} serving as the text encoder. Since the training datasets—RealEstate-10K~\cite{DBLP:journals/tog/ZhouTFFS18}, ACID~\cite{DBLP:conf/iccv/LiuM0SJK21} and DL3DV~\cite{DBLP:conf/cvpr/LingSTZXWYGYLLS24}—do not provide captions, we use PLLAVA~\cite{DBLP:journals/corr/abs-2404-16994} to generate captions for each video clip.

\section{Downstream Tasks Details}

\subsection{Sparse View Interpolation}
\label{sec:svi}
\noindent\textbf{Method Details.} 
We provide a detailed explanation of generating a long-range video in scenarios where the first and last input images have minimal or no overlap. 
Given two input image $\textbf{I}_\text{first}$ and $\textbf{I}_\text{last}$,
we invoke the proposed SCVG to generate the image sequence \( \textbf{x}=\{\textbf{x}_0, \dots, \textbf{x}_{L-1}\} \).
To interpolate those sparse frames to a long dense video, we uniformly sample $m+1$ frames \(\{\textbf{x}_{i_0}, \textbf{x}_{i_1}, \dots, \textbf{x}_{i_m}\} \) from the first-pass result and process the second video generation.
In the second-pass process, each pair of adjacent frames \( (\textbf{x}_{i_j}, \textbf{x}_{i_{j+1}}) \) serves as the input of SCVG and generate $L$ novel views, resulting a long final video.
By adjusting the value of $m$, we can control the length of the final generated video.

\noindent\textbf{Experiment Details.} 
To ensure a fair comparison with ReconX~\cite{DBLP:journals/corr/abs-2408-16767} (32 frames) and ViewCrafter~\cite{DBLP:journals/corr/abs-2409-02048} (25 frames), we set the generated video length to 33 frames. This choice is also influenced by the limitation of the CogVideoX~\cite{DBLP:journals/corr/abs-2408-06072} 3D VAE, which only supports videos with $4n+1$ frames. We filter the training datasets from RealEstate-10K, ACID, and DL3DV-10K to include only videos with at least 33 frames. Furthermore, we remove videos that could not be downloaded and those where the pose counts did not match the frame counts. After these steps, a total of 66,859 videos remain in the final training dataset. For evaluation, we select 100 videos from the test sets of RealEstate-10K and ACID. Following previous methods~\cite{DBLP:journals/corr/abs-2403-14627, DBLP:conf/cvpr/CharatanLTS24, DBLP:journals/corr/abs-2408-16767}, we calculate the evaluation metrics using three frames per clip, specifically the 5th, 15th, and 25th frames.

\subsection{Perpetual View Generation}

\noindent\textbf{Method Details.}
Given the first image $\textbf{I}_\text{first}$ and a pose trajectory, we invoke the proposed SCVG~\cref{alg:code} in an autoregressive manner to generate a sequence of novel views. 
In generating the first clip, the input image $\textbf{I}_\text{first}$ is duplicated to create paired spatial conditioning images for SCVG, aligning with the zero-shot novel view synthesis task in ViewCrafter~\cite{DBLP:journals/corr/abs-2409-02048}. Note that depth predictions from identical images can suffer from scale ambiguity. To align different methods to the same scale for fair comparison, we use DUSt3R~\cite{DBLP:conf/cvpr/Wang0CCR24} to calculate the mean depth of the first image as a reference. We then align the mean depth of the first image from each method to this reference scale. In the subsequent clip generation, we simply use the first and last frames of the previously generated clip as the spatial conditioning pair. 
More sophisticated frame selection strategies can also be employed as alternatives.
% \cam{Each generated image is associated with a depth map, obtained by 3D warping of depth estimates from its spatial conditioning images.
% For each previously generated image serving as a candidate conditioning image, its depth map is warped to all frames in the current clip to calculate the overlap area.
% The two candidates with the largest overlap area are selected as the spatial conditioning images for the current clip.}

\noindent\textbf{Experiment Details.}
Apart from using the datasets detailed in~\cref{sec:svi}, we also evaluate perpetual view generation on the Tanks-and-Temples dataset~\cite{DBLP:journals/tog/KnapitschPZK17} to further validate its generalization capabilities. We use 6 scenes from its test set without utilizing any training data from Tanks-and-Temples.

\subsection{Layout-Conditioned City Generation}
\noindent\textbf{Method Details.} As described in the main paper, we adopt a two-stage approach, primarily integrating different ControlNets. 
The semantic ControlNet output is denoted as $\mathbf{C}^{s}$, 
the depth ControlNet output is $\mathbf{C}^{d}$, 
and the output of our SCVG ControlNet, as described in~\cref{alg:code}, is $\mathbf{C}^{scvg}$.
We combine different ControlNets by linearly weighting their output features.
The weighted and combined features are then added to each block of CogVideoX to produce the output video. 
The distinction between the two stages lies in the combination of these ControlNets.
In the first stage, the features are combined as $\mathbf{\alpha_{1}} \mathbf{C}^{s} + \mathbf{\beta_{1}} \mathbf{C}^{d}$, while in the second stage, they are combined as $\mathbf{\alpha_{2}} \mathbf{C}^{s} + \mathbf{\beta_{2}} \mathbf{C}^{d} + \mathbf{\gamma_{2}} \mathbf{C}^{scvg} $. In our experiments, $\mathbf{\alpha_{1}}$ and $\mathbf{\beta_{1}}$ are both set to 0.5, while $\mathbf{\alpha_{2}}$ and $\mathbf{\beta_{2}}$ are set to 0.3, and $\mathbf{\gamma_{2}}$ is set to 0.4.

\noindent\textbf{Experiment Details.} In this task, we additionally utilize the CityGen dataset from CityDreamer~\cite{DBLP:conf/cvpr/Xie0H024}, which comprises city layout maps derived from OpenStreetMap~\cite{osmdataset} and renderings generated by Google Earth Studio~\cite{google_earth_stdio}. Each trajectory in this dataset contains only 60 frames, while spanning a large scene with a radius of approximately 400 meters, leading to very sparse frame intervals. To address this issue, we use Google Earth Studio to perform frame interpolation on the original trajectories, increasing the number of frames per trajectory to 600. We observe that Google Earth Studio’s mesh-based representation introduces inconsistencies due to misalignment or lighting changes among the images used for mesh reconstruction, leading to artifacts in the training data. For instance, distortions in zebra crossings are frequently observed in the training data. We observe that the artifacts in the training data impact the learning process, as our model also learns and replicates these distortions during training. Despite this, compared to CityDreamer trained on the same data, our model produces significantly better results. 

\begin{figure*}
\centering
\includegraphics[width=1.0\linewidth]{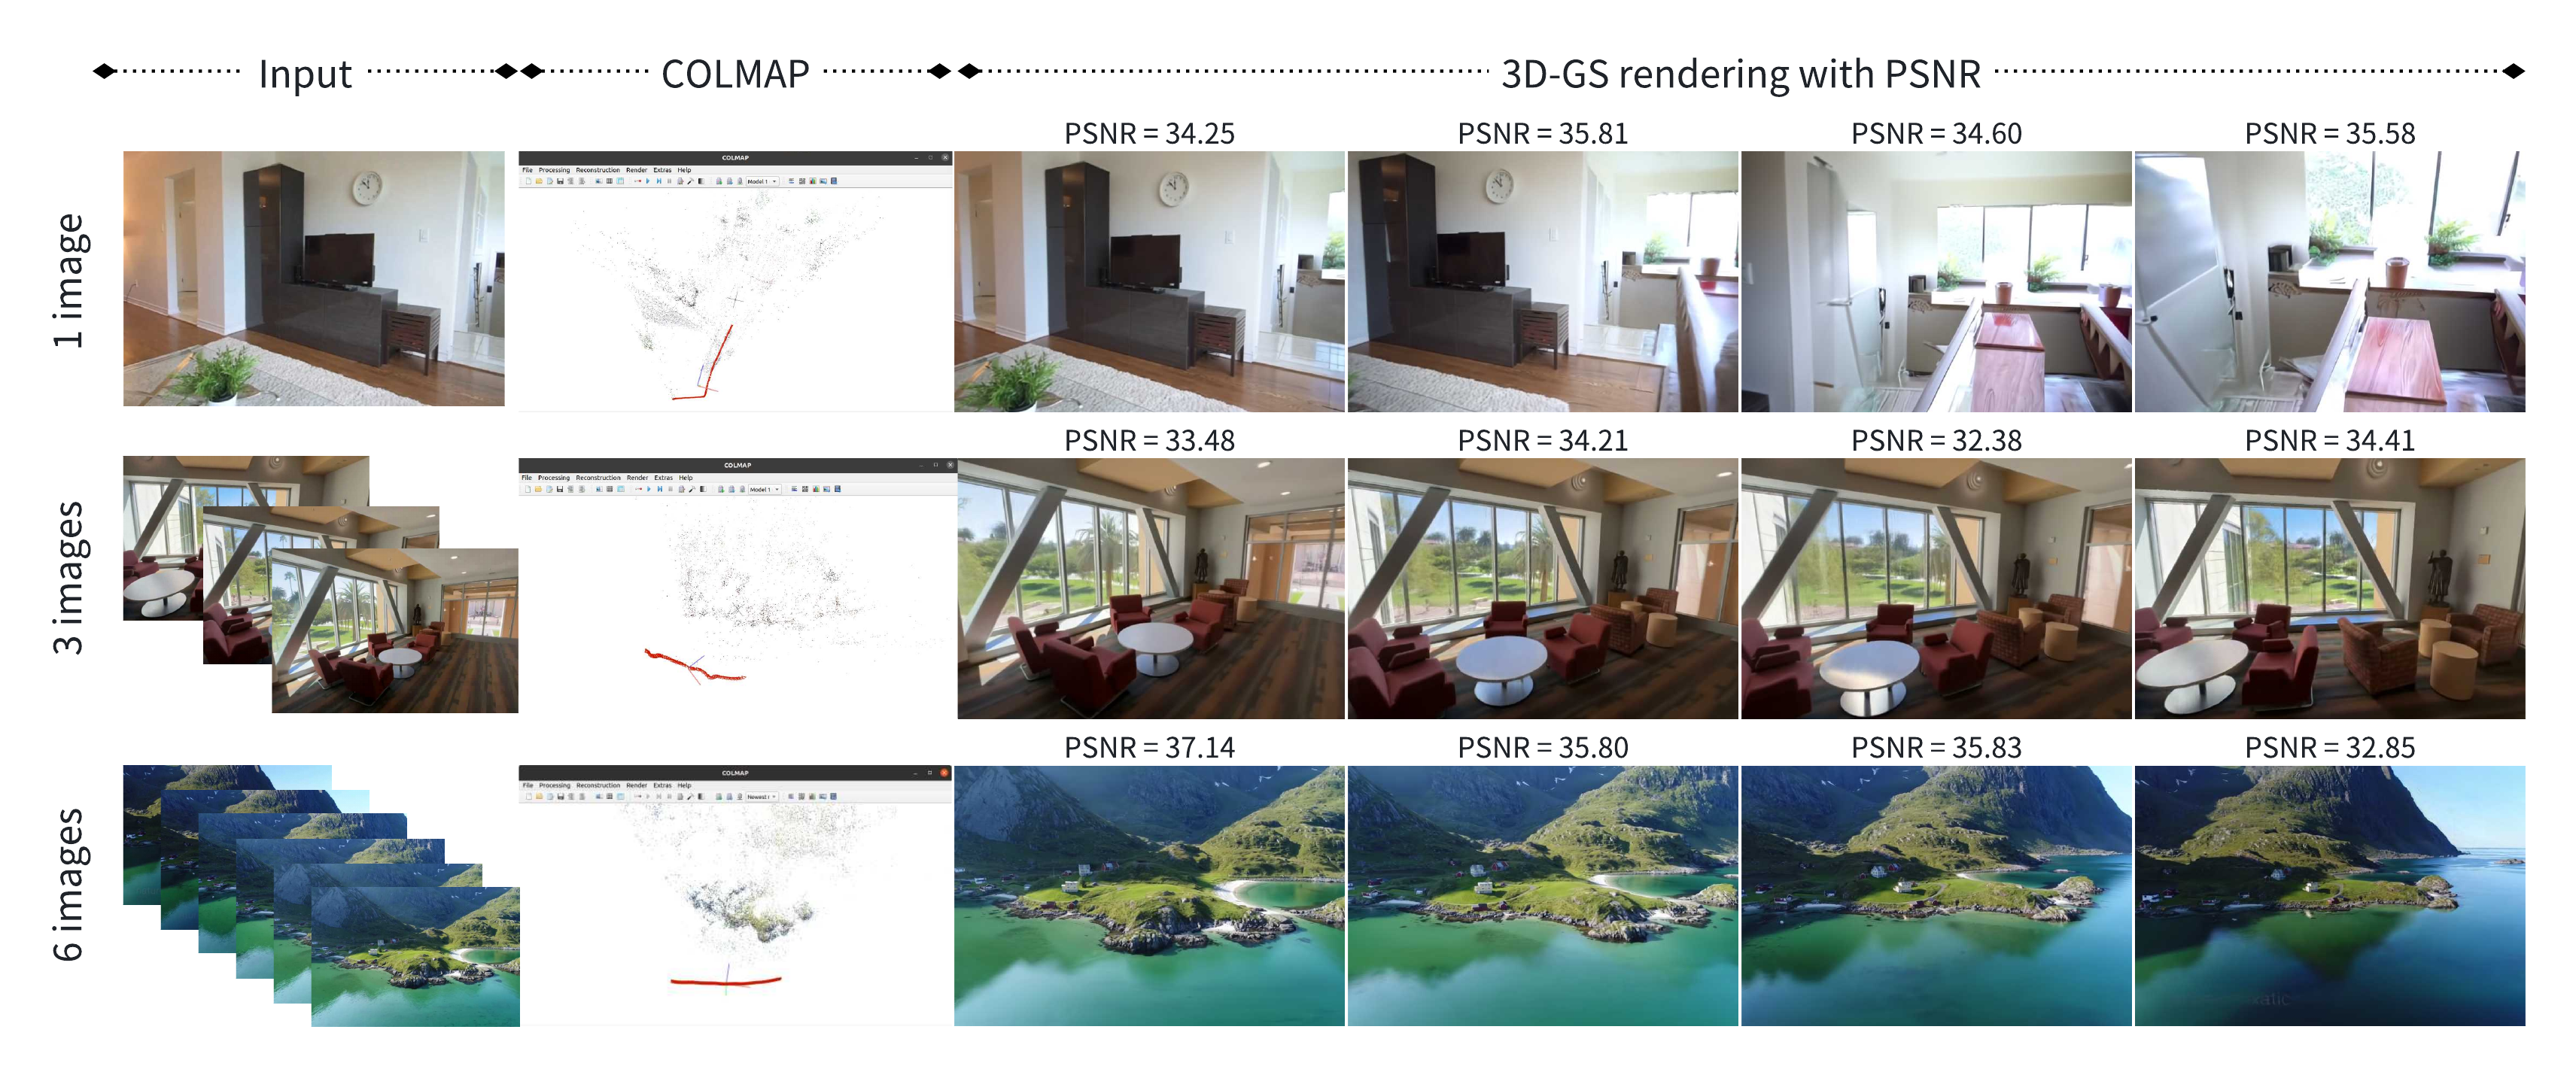}
\caption{
The reconstruction scenes of the generated videos:
the reconstruction scene of single image generated video (the first row);
the scene result interpolated from three images(the second row);
the scene result interpolated from six images(the third row).
}
\label{fig:reconstruction}
\end{figure*}

\section{Evaluation Details}

\subsection{Baselines}

\begin{CJK}{UTF8}{gbsn}
\end{CJK}
The quantitative results for pixelNeRF~\cite{DBLP:conf/cvpr/YuYTK21}, GPNR~\cite{suhail2022generalizable}, AttnRend~\cite{DBLP:conf/iclr/ChenYGYXWK0LL24}, and MuRF ~\cite{DBLP:conf/cvpr/XuCCSZP0024} are sourced from the MVSplat paper~\cite{DBLP:journals/corr/abs-2403-14627}. The results for pixelSplat~\cite{DBLP:conf/cvpr/CharatanLTS24}, MVSplat, GS-LRM~\cite{DBLP:conf/eccv/ZhangBTXZSX24}, DepthSplat~\cite{xu2024depthsplat}, and ReconX ~\cite{DBLP:journals/corr/abs-2408-16767} are taken from their respective original papers. DepthSplat is not evaluated on ACID due to the lack of a released model trained on this dataset. The quantitative results for ViewCrafter~\cite{DBLP:journals/corr/abs-2409-02048}, InfNat0~\cite{DBLP:conf/eccv/LiWSK22}, LucidDreamer ~\cite{DBLP:journals/corr/abs-2311-13384}, MotionCtrl ~\cite{DBLP:conf/siggraph/WangYWLCXLS24}, and CityDreamer~\cite{DBLP:conf/cvpr/Xie0H024}, as well as all qualitative results for each method, are reproduced using their publicly available code.

InfNat0 first resizes input images to \(384 \times 384\) and then crops them to \(256 \times 256\). MotionCtrl resizes images proportionally to a 1024-pixel short side, followed by cropping to \(1024 \times 576\).  We adhere to their default configurations. For LucidDreamer, we crop the input images to square dimensions and resize them to \(512 \times 512\). LucidDreamer supports only predefined camera intrinsics and pose trajectories. We modify the code to accommodate input camera control. Additionally, as LucidDreamer does not support long text prompts, we use text prompts generated with LAVIS ~\cite{DBLP:conf/acl/Li0LWSH23} as specified in their original paper. For ViewCrafter, the images are first cropped to square dimensions and then resized to \(512 \times 288\) to avoid further cropping in ViewCrafter. Since DUSt3R~\cite{DBLP:conf/cvpr/Wang0CCR24} re-estimates camera intrinsics and extrinsics, the resizing process has minimal impact on the final results. 
In perpetual view generation, the necessary code for point cloud stitching is not released. We implement this functionality based on the paper’s description. For the task of layout-conditioned city generation, the results for CityDreamer are obtained by bypassing their unbounded layout generator and instead using our selected layout maps and the same trajectories as input.

\subsection{Metrics}

\noindent\textbf{Short-Range Video Quality.} 
For sparse view interpolation and short-range perpetual view generation, we use the PSNR, SSIM~\cite{DBLP:journals/tip/WangBSS04} and LPIPS~\cite{DBLP:conf/cvpr/ZhangIESW18} to measure the similarity between generated and groundtruth images.
Since different methods for comparison may operate at different resolutions, we consistently resize both the groundtruth and generated images to \(256 \times 256\) for a fair comparison.

\noindent\textbf{Long-Range Video Quality.}
For long-range perpetual view generation, since the output video contains a large amount of generated content, we calculate Fréchet Inception Distance (FID)~\cite{DBLP:conf/nips/HeuselRUNH17} to assess the performance.
For consistent evaluation of generated videos with different lengths, we use a fixed number of images in each FID calculation. Specifically, when calculating FID for generated videos with different lengths, we sample different numbers of clips from the test set to ensure that the total number of frames for each calculation is 5000.
Again, we resize both the groundtruth and generated images to \(256 \times 256\) for a fair comparison.

\noindent\textbf{Pose Accurancy.}
We evaluate the pose-control ability of different methods by comparing the groundtruth poses with estimated poses of the generated images.
In our experiments, we use MASt3R~\cite{DBLP:conf/eccv/LeroyCR24} to estimate poses as it is more robust than traditional methods.
After the pose estimation, we transform the estimated pose to the GT coordinate system and align the scale for evaluation.
Specifically, we first transform the estimated trajectory by aligning the first camera pose to groundtruth, then calculate the scale factor by comparing the lengths of groundtruth and estimated trajectories, and finally apply the scale factor to the estimated trajectories.
We calculate the average rotation error $R_{dist}$ and translation error $T_{dist}$ by:
\begin{equation}
\begin{aligned}
  R_{\text{dist}} &= \frac{1}{n}\sum_{i=1}^{n} \arccos \left( \frac{{\text{tr}(\mathbf{R}_{\text{gen}}^i \mathbf{R}_{\text{gt}}^{iT}) - 1}}{2} \right),\\
  T_{\text{dist}} &= \frac{1}{n}\sum_{i=1}^{n} \left\| \mathbf{T}_{\text{gt}}^i - \mathbf{T}_{\text{gen}}^i \right\|_2,
\end{aligned}
\end{equation}
where $\mathbf{R}_{\text{gen}}^i$ and $\mathbf{T}_{\text{gen}}^i$ are the rotation and translation estimated from the generated video corresponding to the $i$-th frame, while $\mathbf{R}_{\text{gt}}^{i}$ and $\mathbf{T}_{\text{gt}}^i$ are the groundtruth.

For the evaluation of long-range video , considering the computational efficiency of MASt3R, the cost of recovering all frames would be unbearable.
Therefore, we only estimate the poses of keyframes for evaluation.
We select one keyframe from every tenth frame in the first 200 frames of the generated videos, resulting in 21 keyframes $(0, 10, ..., 200)$.

\section{Reconstruction Results}
To further demonstrate the temporal consistency of the long videos generated by the proposed method, we employed COLMAP to perform sparse reconstruction on the generated video sequences and subsequently trained a 3D Gaussian Splatting (3DGS) model.
As illustrated in ~\cref{fig:reconstruction}, both the sparse reconstruction results and the rendered outputs indicate that the generated videos exhibit excellent multi-view consistency, which significantly facilitates the reconstruction of large-scale scenes.
This consistency not only validates the robustness of our method but also highlights its potential for applications requiring high-fidelity scene reconstruction and rendering.

\section{Effect of VDM backbone} 
To ensure a fair comparison with ViewCrafter, we reimplemented its modules using the same CogVideo backbone, eliminating backbone-related discrepancies. 
The key differences between StarGen and ViewCrafter are:
(a) For novel view conditioning, StarGen uses an LRM for latent feature reconstruction, while ViewCrafter relies on DUSt3R for RGB point cloud reconstruction;
(b) StarGen employs ControlNet for condition injection, whereas ViewCrafter uses concatenation.
We evaluated different module combinations under identical experimental settings (Section 4.3, long-range video), benchmarking performance on the RealEstate-10K dataset.
As shown in ~\cref{tab:Ablation_VDM}, our proposed method demonstrates significant advantages even under the same backbone.

\begin{table} 
\centering 
\scalebox{0.68}
{
\begin{tabular}{l|lll|lll}
Method & part (a) & part (b)& backbone & FID$\downarrow$ & $R_\text{dist}$$\downarrow$ & $T_\text{dist}$$\downarrow$ \\
\midrule
 Ours & LRM & CN & CogVideo & \textbf{41.72} & \textbf{2.088} & \textbf{0.453} \\
 DUSt3R+CN & DUSt3R & CN & CogVideo & 55.14 & \underline{2.580} & \underline{0.694} \\
 DUSt3R+Concat & DUSt3R    & Concat & CogVideo & \underline{51.40} & 2.739 & 0.716 \\
 ViewCrafter & DUSt3R    & Concat & DynamicCrafter & 62.91 & 11.32 & 0.86
\end{tabular}
}
\caption{Ablation results for different module combinations. 
}
\label{tab:Ablation_VDM}
\end{table}
